# Supplementary material for: Single-photon embedded eigenstates in coupled cavity-atom systems
Source: arXiv:1805.03287 ancillary file (2018-05-08)
Supplement: Supplementary file 1 [file Supplementary_Material.pdf]

Supplemental Material for

# Single-photon embedded eigenstates in coupled cavity-atom systems

Michele Cotrufo[1,§] and Andrea Alù[1,2,3,4,*]

[1]*Department of Electrical and Computer Engineering, The University of Texas at Austin, Austin, TX 78712, USA*

[2]*Photonics Initiative, Advanced Science Research Center, City University of New York, New York 10031, USA*

[3]*Physics Program, Graduate Center, City University of New York, New York 10016, USA*

[4]*Department of Electrical Engineering, City College of The City University of New York, New York 10031, USA*

[§] michele.cotrufo@utexas.edu, [*]aalu@gc.cuny.edu

## 1. Derivation of the EE condition for the atom-cavity system

In the main text, we considered the full Hamiltonian of the atom-cavity-waveguide system,

$$\hat{H} = \hat{H}_{AC} + \int_{-\infty}^{+\infty} dk\ \omega_k \hat{c}_k^\dagger \hat{c}_k + \int_{-\infty}^{+\infty} dk \left[ \hat{c}_k^\dagger (V_C \hat{a} + V_A \hat{\sigma}_-) + h.c. \right] \tag{S1}$$

where $\hat{H}_{AC} = \omega_c \hat{a}^\dagger \hat{a} + \omega_A \hat{\sigma}_+ \hat{\sigma}_- + J\left(\hat{a}\hat{\sigma}_+ + h.c.\right)$, and we showed that a single-excitation state $|\Psi_{EE}^{(1)}\rangle = C^{(1)}|1,g\rangle + A^{(1)}|0,e\rangle$ is an embedded eigenstate (EE) if $V_C C^{(1)} + V_A A^{(1)} = 0$. We show here that the condition $V_C C^{(1)} + V_A A^{(1)} = 0$ is equivalent to the EE condition in eq. 1 of the main text (with the parameters relabeled accordingly). In the one-excitation sector, we can rewrite the time-independent Schroedinger equation $\hat{H}_{AC}|\Psi_{EE}^{(1)}\rangle = \omega_{EE}^{(1)}|\Psi_{EE}^{(1)}\rangle$ as

$$\begin{pmatrix} \omega_A & J \\ J & \omega_C \end{pmatrix} \begin{pmatrix} A^{(1)} \\ C^{(1)} \end{pmatrix} = \omega_{EE}^{(1)} \begin{pmatrix} A^{(1)} \\ C^{(1)} \end{pmatrix}. \tag{S2}$$

Replacing $C^{(1)} = -V_A / V_C A^{(1)}$ we obtain two equations for $\omega_{EE}^{(1)}$, and by requiring that they both hold we obtain

$$\frac{\omega_A V_c - J V_A}{V_C} = \frac{\omega_C V_A - J V_C}{V_C} \Rightarrow J(V_A^2 - V_C^2) = (\omega_A - \omega_C) V_A V_C. \tag{S3}$$

## 2. Derivation of the Input-Output formalism for the atom-cavity Hamiltonian

In this section we derive the input-output formalism for the system considered in the main text. The derivation follows closely the one outlined in ref. [1]. We start by considering the Hamiltonian in eq. (S1). We can split the waveguide modes into right- and left-propagating modes

$$\int_{-\infty}^{+\infty} dk\ \omega_k \hat{c}_k^\dagger \hat{c}_k = \int_{0}^{+\infty} dk\ \omega_k \hat{c}_k^\dagger \hat{c}_k + \int_{-\infty}^{0} dk\ \omega_k \hat{c}_k^\dagger \hat{c}_k \tag{S4}$$

Next, we assume that the waveguide dispersion relation can be linearized in a narrow frequency range centered around a frequency of interest $\omega_0$. This allows us to write $\omega_k = \omega_0 + v_g(k-k_0)$ for $k>0$, and $\omega_k = \omega_0 - v_g(k+k_0)$ for $k<0$, where $\pm k_0$ is the wavevector at $\omega_0$ and $v_g$ is the group velocity. By defining the operators $\hat{c}_{R,\omega} \equiv \hat{c}_{k+k_0}/\sqrt{v_g}$ , $\hat{c}_{L,\omega} \equiv \hat{c}_{k-k_0}/\sqrt{v_g}$ , and extending the limits of integration to $\pm\infty$, the free evolution Hamiltonian of the waveguide modes becomes

$$H_{WG} = \int_{-\infty}^{+\infty} d\omega\, \omega\, (\hat{c}_{R,\omega}^\dagger \hat{c}_{R,\omega} - \hat{c}_{L,\omega}^\dagger \hat{c}_{L,\omega}) \tag{S5}$$

where we note that the frequency $\omega$ is now defined with respect to $\omega_0$. By substituting the new operators in the full Hamiltonian in eq. (S1) we get

$$\hat{H} = \hat{H}_{AC} + \int_{-\infty}^{+\infty} d\omega\, \omega\, (\hat{c}_{R,\omega}^\dagger \hat{c}_{R,\omega} - \hat{c}_{L,\omega}^\dagger \hat{c}_{L,\omega}) + \frac{1}{\sqrt{v_g}} \int_{-\infty}^{+\infty} d\omega \left[ (\hat{c}_{R,\omega}^\dagger + \hat{c}_{L,\omega}^\dagger)(V_C \hat{a} + V_A \hat{\sigma}_-) + h.c. \right] \tag{S6}$$

where we also subtracted the frequency $\omega_0$ in the atom-cavity Hamiltonian,

$\hat{H}_{AC} = (\omega_c - \omega_0)\hat{a}^\dagger \hat{a} + (\omega_A - \omega_0)\hat{\sigma}_+ \hat{\sigma}_- + J\left(\hat{a}\hat{\sigma}_+ + h.c.\right)$. From the Hamiltonian in eq. (S6) we can derive the Heisenberg equations of motion of the different operators,

$$\dot{\hat{c}}_{R,\omega} = -i\omega \hat{c}_{R,\omega} - i\frac{1}{\sqrt{v_g}}\left(V_A \hat{\sigma}_- + iV_C \hat{a}\right) \tag{S7}$$

$$\dot{\hat{c}}_{L,\omega} = i\omega \hat{c}_{R,\omega} - i\frac{1}{\sqrt{v_g}}\left(V_A \hat{\sigma}_- + iV_C \hat{a}\right) \tag{S8}$$

$$\dot{\hat{\sigma}}_- = -i(\omega_A - \omega_0)\hat{\sigma}_- + iJ\hat{a}\hat{\sigma}_z + i\frac{V_A^*}{\sqrt{v_g}}\hat{\sigma}_z \int d\omega (\hat{c}_{R,\omega}^\dagger + \hat{c}_{L,\omega}^\dagger) \tag{S9}$$

$$\dot{\hat{a}} = -i(\omega_C - \omega_0)\hat{a} - iJ\hat{\sigma}_- - i\frac{V_C^*}{\sqrt{v_g}} \int d\omega (\hat{c}_{R,\omega}^\dagger + \hat{c}_{L,\omega}^\dagger)\ . \tag{S10}$$

We can formally integrate eqs. (S7) and (S8),

$$\hat{c}_{R/L,\omega}(t) = \hat{c}_{R/L,\omega}(t_0) e^{\mp i\omega(t-t_0)} - \frac{i}{\sqrt{v_g}} \int_{t_0}^{t} dt' e^{\mp i\omega(t-t')} [V_A \hat{\sigma}_-(t') + V_C \hat{a}(t')] \tag{S11}$$

and substitute them into eqs. (S9) and (S10), obtaining

$$\dot{\hat{\sigma}}_- = -i\left(\omega_A - \omega_0 - i2\pi\frac{|V_A|^2}{v_g}\right)\hat{\sigma}_- + i\left(J - i2\pi\frac{V_A^* V_C}{v_g}\right)\hat{a}\hat{\sigma}_z + i\sqrt{\frac{2\pi}{v_g}}V_A^{\ *}\hat{\sigma}_z[\hat{c}_{R,IN}(t) + \hat{c}_{L,IN}(t)] \quad \text{(S12)}$$

$$\dot{\hat{a}} = -i\left(\omega_C - \omega_0 - i2\pi\frac{|V_C|^2}{v_g}\right)\hat{a} - i\left(J - i2\pi\frac{V_C^* V_A}{v_g}\right)\hat{\sigma}_- - i\sqrt{\frac{2\pi}{v_g}}V_C^{\ *}[\hat{c}_{R,IN}(t) + \hat{c}_{L,IN}(t)] \quad \text{(S13)}$$

where we have reversed the order of integration and we used $\int d\omega \exp[\pm i\omega(t-t')] = 2\pi\delta(t-t')$. Following a well-known procedure [1], we have defined the input fields as

$$\hat{c}_{R/L,IN}(t) = \frac{1}{\sqrt{2\pi}}\int d\omega\, \hat{c}_{R/L,\omega}(t_0)e^{\mp i\omega(t-t_0)} \quad \text{(S14)}$$

where $t_0$ is an arbitrary initial time. Equations (S12) and (S13) show explicitly that the presence of the waveguide, besides providing an input channel for the system, leads to finite decay rates for the atom and cavity amplitudes, $\Gamma_{A,C} = 2\pi |V_{A/C}|^2 / v_g$ , and to a modification of the bare coupling rate $J$ .

### 3. Eigenstates of the atom-cavity system in the one- and two-excitation sector

Equations (S12)-(S13) allows us to calculate the eigenstates and complex eigenvalues of the atom-cavity system in absence of external pumping. Indeed, the obtained equations of motion are equivalent to a non-Hermitian effective Hamiltonian

$$\hat{H}_{AC}^{(eff)} = (\omega_c - i\Gamma_C)\hat{a}^\dagger\hat{a} + (\omega_A - i\Gamma_A)\hat{\sigma}_+\hat{\sigma}_- + (J - i\sqrt{\Gamma_C\Gamma_A})\left(\hat{a}\hat{\sigma}_+ + h.c.\right) \quad \text{(S15)}$$

where we assumed the couplings $V_{A/C}$ to be real, and we have removed the common frequency $\omega_0$. Therefore, we can find the eigenstates and eigenvalues in the one-excitation subspace by diagonalizing the matrix

$$\begin{pmatrix} \omega_A - i\Gamma_A & J - i\sqrt{\Gamma_C\Gamma_A} \\ J - i\sqrt{\Gamma_C\Gamma_A} & \omega_C - i\Gamma_C \end{pmatrix} \quad \text{(S16)}$$

with the additional requirement given by eq. (S3). A direct calculation gives the frequencies of the EE and of the bright mode

$$\omega_{EE}^{(1)} = \omega_C - J\frac{V_C}{V_A} = \omega_A - J\frac{V_A}{V_C} \ , \quad \text{(S17)}$$

$$\tilde{\omega}_B^{(1)} = \omega_A + J\frac{V_C}{V_A} - i\pi\frac{V_A^2 + V_C^2}{v_g} = \omega_C + J\frac{V_C}{V_A} - i\pi\frac{V_A^2 + V_C^2}{v_g} \quad \text{(S18)}$$

We note that, according to the sign of $J\,V_C/V_A$, the EE will be the lower ($JV_C/V_A>0$) or upper ($J\,V_C/V_A<0$) resonance, in agreement with the original discussion of Friedrich and Wintgen [2]. In the following, and in the main text, we indicate the complex frequency of the single-photon bright mode as $\tilde{\omega}_B^{(1)} \equiv \omega_B^{(1)} - i\Gamma$. The corresponding eigenstates are $|\Psi_{EE}^{(1)}\rangle = N\,(V_C\hat{\sigma}_+ - V_A\hat{a}^\dagger)\,|0\rangle$ and $|\Psi_B^{(1)}\rangle = N\,(V_A\hat{\sigma}_+ + V_C\hat{a}^\dagger)\,|0\rangle$, with the normalization constant $N = 1/\sqrt{V_A^2+V_C^2}$ .

Similarly, we can look for the eigenstates of the system in the two-excitation sector, where a general state can be written as $|\Psi^{(2)}\rangle = \left[E_{2C}(\hat{a}^{\dagger 2}/\sqrt{2}) + E_{AC}\hat{a}^\dagger\hat{\sigma}_+\right]|0\rangle$. The eigenvalues and eigenstates are therefore obtained by diagonalizing the matrix

$$\begin{pmatrix} \omega_A+\omega_C-i(\Gamma_A+\Gamma_C) & \sqrt{2}\left[J-i\sqrt{\Gamma_C\Gamma_A}\right] \\ \sqrt{2}\left[J-i\sqrt{\Gamma_C\Gamma_A}\right] & 2(\omega_C-i\Gamma_C) \end{pmatrix} \tag{S19}$$

The eigenvalues and eigenstates do not have a simple form in this case, and they are not reported here. We note that both eigenvalues $\tilde{\omega}_{1/2}^{(2)} = \omega_{1/2}^{(2)} - i\Gamma_{1/2}^{(2)}$ have a nonzero imaginary component (as expected since no EE exists in the two-excitation sector), and their ratio reads

$$\frac{\Gamma_1^{(2)}}{\Gamma_2^{(2)}} = \frac{5}{4} + \frac{3}{2\alpha^2} + \frac{1}{4\alpha^4} + \frac{1+3\alpha^2}{4\alpha^4}\sqrt{\alpha^4+6\alpha^2+1}, \tag{S20}$$

where we have set $\alpha = V_C/V_A$. We note that for $\alpha = O(1)$ the two decay rates are quite different. For example, for $\alpha = 1$, $\Gamma_1^{(2)}/\Gamma_2^{(2)} \approx 5.8$, and for $\alpha = 0.5$ (the value used in figs. 1d, 2(a,b,d), 3 and 4a of the main text), $\Gamma_1^{(2)}/\Gamma_2^{(2)} \approx 22$. Therefore, also in the two-excitation sector we can identify a “bright” and a “dark” eigenstate, whose real frequencies are denoted $\omega_B^{(2)}$ and $\omega_D^{(2)}$, respectively, in fig. 2d of the main text.

## 4. Derivation of a density-matrix master equation from the input-output theory

In order to calculate numerically the dynamics of the system, it is useful to recast Eqs. (S12) and (S13) into a master equation for the density matrix (in Schrödinger representation) of the atom-cavity system. We start from a standard form of the master equation

$$\dot{\rho} = -i[\hat{H}_{AC} + \hat{H}_{input}, \rho] + \mathcal{L}\rho\mathcal{L}^\dagger - \{\mathcal{L}\mathcal{L}^\dagger, \rho\}/2 \tag{S21}$$

where $\rho$ is the density matrix of the atom-cavity system, $\hat{H}_{input} = \sqrt{2\pi/v_g}\,[(V_a\hat{\sigma}_- + V_c\hat{a})(\hat{c}_{R,IN}(t) + \hat{c}_{L,IN}(t)) + h.c.]$ and $\mathcal{L}$ is a Lindblad operator to be found. The operator $\mathcal{L}$ is necessary to describe the non-unitary evolution introduced by the waveguide through the decay rates $\Gamma_{A,C}$ and the modification of the coupling $J$. To determine the exact form of $\mathcal{L}$ we exploit the

fact that the master equation in Schrödinger representation [eq. (S21)] can be expressed in Heisenberg representation for a general observable $\hat{x}$ as

$$\dot{\hat{x}} = i[\hat{H}_{AC} + \hat{H}_{input}, \hat{x}] + \mathcal{L}^{\dagger} x \mathcal{L} - \{\mathcal{L}\mathcal{L}^{\dagger}, \rho\}/2 . \tag{S22}$$

Therefore, the operator $\mathcal{L}$ must be chosen such that ,when eq. (S22) is applied to the operators $\hat{\sigma}_-$ and $\hat{a}$ , the equations of motions (S12) and (S13) are obtained. By starting with the Ansatz $\mathcal{L} = A\hat{a} + B\hat{\sigma}_-$, it is straightforward to find that $\mathcal{L} = \sqrt{4\pi / v_g}(V_A \hat{a} + V_C \hat{\sigma}_-)$ .

The results shown in fig. 1d and 4c of the main paper have been obtained by solving numerically the density matrix in eq. (S21) with the aid of the open-source Python framework QuTip [3]. Similarly to what we do in the main text for the two-photon excitation, we assumed an identical excitation in the right and left channel, and we define the even input mode, $\hat{c}_{e,IN}(t) \equiv \left[\hat{c}_{R,IN}(t) + \hat{c}_{L,IN}(t)\right]/\sqrt{2}$ . Moreover, we assume that the input field is a wave-packet in a coherent state with an average photon number $\langle N \rangle$ . This allows us to replace the operator $\hat{c}_{e,IN}(t)$ by $\langle N \rangle \xi(t)$ where $\xi(t)$ is a square-normalized scalar function. In particular, for the calculations in fig. 1d and 4c of the main paper we considered a Gaussian wave-packet $\xi(t) = (\pi\sigma^2)^{1/4} \exp[-(t-t_0)^2/(2\sigma^2) + i\omega t]$.

## 5. Dynamical equations in the two-photon sector

In this section we derive the differential equations that describe the time-evolution of an arbitrary two-excitation initial state of the atom-cavity-waveguide system, and we subsequently recast them in a form that facilitates the analytical and numerical calculations. We note that a similar technique has been used in ref. [4] for the case of a single atom. We start by showing again the total Hamiltonian of the system (eq. 4 of the main text)

$$\hat{H}_e = \hat{H}_{AC} - i\int dx\, \hat{c}_e^{\dagger}(x)\, \partial_x\, \hat{c}_e(x) + \int dx \delta(x) \left[\hat{c}_e^{\dagger}(x)(\tilde{V}_C \hat{a} + \tilde{V}_A \hat{\sigma}_-) + h.c.\right] \tag{S23}$$

and the general form of a two-photon state,

$$\begin{aligned} |\psi(t)\rangle = \Big[ & \int dx_1 dx_2 \chi(x_1, x_2, t) \hat{c}_e^{\dagger}(x_1) \hat{c}_e^{\dagger}(x_2)/\sqrt{2} + \int dx \left(\phi_A(x,t)\hat{\sigma}_+ + \phi_C(x,t)\hat{a}^{\dagger}\right)\hat{c}_e^{\dagger}(x) + \\ & E_{AC}(t)\hat{a}^{\dagger}\hat{\sigma}_+ + E_{2C}(t)(\hat{a}^{\dagger})^2/\sqrt{2}\Big] |0\rangle \end{aligned} \tag{S24}$$

where the meaning of all functions is defined in the main text. Consistently with the main text we have set $v_g = 1$ and $\tilde{V}_{A/C} \equiv 2\sqrt{\pi}\, V_{A/C}$. We now apply the time-dependent Schrödinger equation $i\partial_t |\psi\rangle = \hat{H}_e |\psi\rangle$ and we equate the coefficients of each vector state. This leads to five differential equations,

$$\begin{cases} \partial_t \chi(x_1,x_2,t) = -(\partial_{x_1}+\partial_{x_2})\chi(x_1,x_2,t) - \\ \qquad -i\frac{\tilde{V}_A}{\sqrt{2}}\left[\phi_A(x_1,t)\delta(x_2)+\phi_A(x_2,t)\delta(x_1)\right] - i\frac{\tilde{V}_C}{\sqrt{2}}\left[\phi_C(x_1,t)\delta(x_2)+\phi_C(x_2,t)\delta(x_1)\right], \\ \partial_t\phi_A(x,t) = -\partial_x\phi_A(x,t) - i(\omega_A-\omega_0)\phi_A(x,t) - iJ\phi_C(x,t) - \\ \qquad -i\frac{\tilde{V}_A^*}{\sqrt{2}}[\chi(x,0,t)+\chi(0,x,t)] - i\delta(x)\tilde{V}_C E_{AC}(t), \\ \partial_t\phi_C(x,t) = -\partial_x\phi_C(x,t) - i(\omega_C-\omega_0)\phi_C(x,t) - iJ\phi_A(x,t) - \\ \qquad -i\frac{\tilde{V}_C^*}{\sqrt{2}}[\chi(x,0,t)+\chi(0,x,t)] - i\delta(x)\left(\tilde{V}_A E_{AC}(t)+\sqrt{2}\tilde{V}_C E_{2C}(t)\right), \\ \partial_t E_{2C}(t) = -2i(\omega_C-\omega_0)E_{2C}(t) - i\sqrt{2}JE_{AC}(t) - i\sqrt{2}\tilde{V}_C^*\phi_C(0,t), \\ \partial_t E_{AC}(t) = -i(\omega_C+\omega_A-2\omega_0)E_{AC}(t) - i\sqrt{2}JE_{2C}(t) - i\left[\tilde{V}_C^*\phi_A(0,t)+\tilde{V}_A^*\phi_C(0,t)\right]. \end{cases} \quad \text{(S25)}$$

In principle, these five inter-dependent differential equations must be solved simultaneously to describe correctly the system dynamics. However, the system can be largely simplified by formally integrating the equation for $\partial_t\chi(x_1,x_2,t)$ with the aid of the Fourier transform, which leads to

$$\begin{aligned} &\chi(x_1,x_2,t) = \chi(x_1-t,x_2-t,0) - \\ &-i\left[\frac{\tilde{V}_A}{\sqrt{2}}\left[\phi_A(x_1-x_2,t-x_2)\theta(x_2)\theta(t-x_2)+\phi_A(x_2-x_1,t-x_1)\theta(x_1)\theta(t-x_1)\right] + A\leftrightarrow C\right], \end{aligned} \quad \text{(S26)}$$

that is, the two-photon function $\chi(x_1,x_2,t)$ is given by its value at $t=0$ (shifted by the photon propagation time) plus a term that depends on the values of $\phi_A$ and $\phi_C$ at different positions and times. By replacing eq. (S26) in the differential equations for $\partial_t\phi_A$ and $\partial_t\phi_C$ we get

$$\begin{cases} \partial_t\phi_A(x,t) = -\partial_x\phi_A(x,t) - i\left(\omega_A-\omega_0-i\frac{|\tilde{V}_A|^2}{2}\right)\phi_A(x,t) - i\left(J-i\frac{\tilde{V}_A^*\tilde{V}_C}{2}\right)\phi_C(x,t) - \\ \qquad -\theta(-x)\theta(t-x)\left[|\tilde{V}_A|^2\,\phi_A(-x,t-x)+\tilde{V}_A^*\tilde{V}_C\phi_C(-x,t-x)\right] \\ \qquad -i\frac{\tilde{V}_A^*}{\sqrt{2}}[\chi(x-t,-t,0)+\chi(-t,x-t,0)] - i\delta(x)\tilde{V}_C E_{AC}(t), \\ \partial_t\phi_C(x,t) = -\partial_x\phi_C(x,t) - i\left(\omega_C-\omega_0-i\frac{|\tilde{V}_C|^2}{2}\right)\phi_C(x,t) - i\left(J-i\frac{\tilde{V}_C^*\tilde{V}_A}{2}\right)\phi_A(x,t) - \\ \qquad -\theta(-x)\theta(t-x)\left[|\tilde{V}_C|^2\,\phi_C(-x,t-x)+\tilde{V}_C^*\tilde{V}_A\phi_C(-x,t-x)\right] \\ \qquad -i\frac{\tilde{V}_C^*}{\sqrt{2}}[\chi(x-t,-t,0)+\chi(-t,x-t,0)] - i\delta(x)\left(\tilde{V}_A E_{AC}(t)+\sqrt{2}\tilde{V}_C E_{2C}(t)\right). \end{cases} \quad \text{(S27)}$$

By comparing eqs. (S27) with eqs. (S25) we note that the time evolution of $\phi_A(x,t)$ and $\phi_C(x,t)$ now depends only on the values of $\chi(x_1,x_2,t)$ at $t=0$, and additional terms appeared: in the first row of both

eqs. (S27) the frequencies and coupling strength $J$ have been modified, similarly to what happened in eqs. (S12) and (S13). Moreover, the second lines of both eqs. (S27) contain nonlocal terms that are nonzero for $0<x<t$ and depend on the values of $\phi_A(x,t)$ and $\phi_C(x,t)$ in the region $x<0$. These terms describe processes where the cavity or the atom first emits a photon and later absorbs another photon. An example of these processes is shown in fig. S1: at a certain time, a photon is in the waveguide at $x<0$ and the atom is excited; The atom can emit a photon that starts travelling towards $+x$, thus feeding the two photon state. When the first photon arrives at $x=0$ it excites again the atom, and therefore it re-transfers the excitation from the two-photon state to the $\hat{c}_e^\dagger(x)\hat{\sigma}_+|0\rangle$ state.

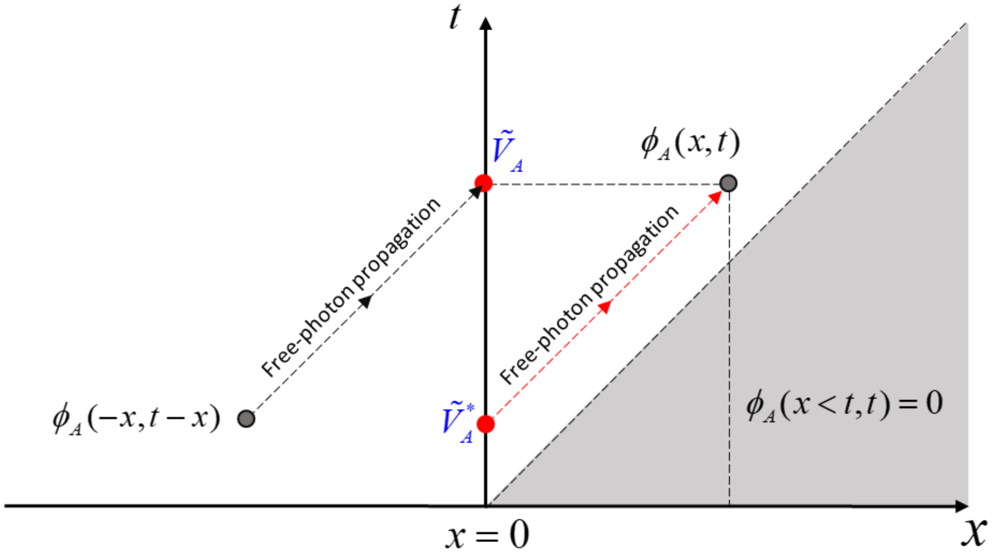


**Figure S1.** Schematic description of the nonlocal term $|\tilde{V}_A|^2\,\phi_A(-x,t-x)$ in the first of eqs. (S27), which makes the field $\phi_A$ at $(x,t)$ dependent on the value of the same field at $(-x,t-x)$. At time $t-x$, there is an amplitude probability equal to $\phi_A(-x,t-x)$ to have one photon at $-x$ and the atom excited. The atom decays into the waveguide with amplitude probability weighted by $\tilde{V}_A^*$, creating a photon that propagates freely (red dashed arrow) to the point $(x,t)$. This process feeds the two-photon amplitude probability. Simultaneously, the photon that was at position $-x$ propagates freely (black dashed arrow) to the point $(0,t)$, where it is absorbed by the atom with an amplitude probability weighted by $\tilde{V}_A$. The overall process creates a state with the atom excited and a photon in the waveguide at position $x$, thus "feeding" the field $\phi_A(x,t)$ with a probability amplitude weighted by $|\tilde{V}_A|^2$. Similar explanations hold for the other nonlocal terms in eqs. (S27)

A further simplification of the dynamical equations (S25) is obtained by noticing that the equations for $\partial_t E_{2C}(t)$ and $\partial_t E_{AC}(t)$ depend only on the values of $\phi_A(x,t)$ and $\phi_C(x,t)$ at $x=0$. Since these two

functions are discontinuous at $x=0$, we set $\phi_{A/C}(0,t)=[\phi_{A/C}(0^+,t)+\phi_{A/C}(0^-,t)]/2$. By integrating in space the eqs. for $\phi_A(x,t)$ and $\phi_C(x,t)$ in (S25) in the interval $[0-\epsilon,0+\epsilon]$, and taking the limit $\epsilon\to 0^+$, we find the boundary conditions

$$\begin{aligned}&\phi_A(0^+,t)=\phi_A(0^-,t)-i\tilde{V}_C E_{AC}(t),\\&\phi_C(0^+,t)=\phi_C(0^-,t)-i\left(\tilde{V}_A E_{AC}(t)+\sqrt{2}\tilde{V}_C E_{2C}(t)\right).\end{aligned}\tag{S28}$$

Plugging these results into the eqs. for $\partial_t E_{2C}(t)$ and $\partial_t E_{AC}(t)$ we get

$$\begin{cases}\partial_t E_{2C}(t)=-2i\left(\omega_C-\omega_0-i\dfrac{|\tilde{V}_C|^2}{2}\right)E_{2C}(t)-i\sqrt{2}\left(J-i\dfrac{\tilde{V}_C^*\tilde{V}_A}{2}\right)E_{AC}(t)-i\sqrt{2}\tilde{V}_C^*\phi_C(0^-,t),\\ \partial_t E_{AC}(t)=-i\left(\omega_C+\omega_A-2\omega_0-i\dfrac{|\tilde{V}_C|^2+|\tilde{V}_A|^2}{2}\right)E_{AC}(t)-i\sqrt{2}\left(J-i\dfrac{\tilde{V}_C^*\tilde{V}_A}{2}\right)E_{2C}(t)-i\left[\tilde{V}_C^*\phi_A(0^-,t)+\tilde{V}_A^*\phi_C(0^-,t)\right],\end{cases}\tag{S29}$$

where, again, the influence of the waveguide on the decay rates and on the atom-cavity coupling is now shown explicitly.

The form of the equations (S27) and (S29) allows to apply a straightforward (analytical or numerical) method of solution (as also discussed in [4]). First, equations (S27) are solved for $x<0$ and arbitrary $t\geq 0$. In this region, the terms proportional to $\theta(-x)\theta(t-x)$ and $\delta(x)$ are zero. Additionally, when there is no two-photon initial state [i.e., $\chi(x_1,x_2,0)=0$] an analytical solution is always possible (see next section). Next, we use the values of $\phi_A(x,t)$ and $\phi_C(x,t)$ at $x=0^-$ to solve for $E_{2C}(t)$ and $E_{AC}(t)$ by using eqs. (S29). Finally, we solve for $\phi_A(x,t)$ and $\phi_C(x,t)$ in the region $0<x<t$ by using the boundary conditions in eqs. (S28). In this step, the terms proportional to $\theta(-x)\theta(t-x)$ in eqs. (S27) have been fully calculated in the first step. We also note that, by causality, $\phi_A(x,t)=\phi_C(x,t)=0$ for $x>t$ (if we assume that at $t=0$ no photon was present in the waveguide for $x>0$).

The calculations shown in the main text (figs. 2, 3 and 4a) have been obtained by solving numerically eqs. (S27) and (S29) with a home-built leapfrog FDTD algorithm, similar to the one outlined in ref. [5] (but generalized to the case of one atom and a cavity).

## 6. Efficiency of the release process, analytical results

In this section we first derive analytical results for the process in which the EE is released, and later we seek for conditions to achieve a perfect release. To simplify the notation, in this section we re-label $\tilde{V}_{A/C}\to V_{A/C}$. We consider an initial state in which the atom-cavity system contains one excitation in the EE and one photon is in the waveguide in the region $x<0$. The initial state is therefore

$$|\psi(t=0)\rangle=\int dx F(x)\hat{c}^\dagger(x)|\Psi_{EE}^{(1)}\rangle,\tag{S30}$$

where $|\Psi_{EE}^{(1)}\rangle=(V_C^2+V_A^2)^{-1/2}\cdot(V_c\hat{\sigma}_+-V_A\hat{a}^\dagger)|0\rangle$ and $F(x)$ is a square-normalized function that describes the spatial shape of the single-photon pulse, with $F(x>0)=0$. Therefore, to obtain the system evolution,

we need to solve eqs. (S27) and (S29) with the initial conditions $\phi_A(x,0) = \left(V_C / \sqrt{V_C^2 + VA^2}\right) F(x)$ and $\phi_C(x,0) = -\left(V_A / \sqrt{V_C^2 + VA^2}\right) F(x)$. For $x < 0$, and assuming that the system is set in the EE condition, the evolution of the fields $\phi_A$ and $\phi_C$ is simply given by

$$\begin{aligned} \phi_A(x<0,t) &= \frac{V_C}{\sqrt{V_C^2 + VA^2}} e^{-i\omega_{EE}t} F(x-t) \\ \phi_C(x<0,t) &= -\frac{V_A}{\sqrt{V_C^2 + VA^2}} e^{-i\omega_{EE}t} F(x-t) \end{aligned} \tag{S31}$$

where $\omega_{EE}$ is the frequency of the embedded eigenstate. The time evolution of $E_{2C}(t)$ and $E_{AC}(t)$ is then obtained from eqs. (S29), resulting in the linear system

$$\partial_t \begin{pmatrix} E_{2C} \\ E_{AC} \end{pmatrix} = -i \begin{pmatrix} 2(\omega_C - \omega_0) - iV_C^2 & \sqrt{2}\tilde{J} \\ \sqrt{2}\tilde{J} & \omega_C + \omega_A - 2\omega_0 - i(V_A^2 + V_C^2)/2 \end{pmatrix} + i \begin{pmatrix} \sqrt{2}V_C V_A \\ V_A^2 - V_C^2 \end{pmatrix} \frac{F(-t)e^{-i\omega_{EE}t}}{\sqrt{V_A^2 + V_C^2}} \tag{S32}$$

which can be solved with standard techniques (for brevity we have defined $\tilde{J} = J - iV_A V_C / 2$). The general solution (assuming $E_{2C}(0) = E_{AC}(0) = 0$) has the form

$$\begin{pmatrix} E_{2C}(t) \\ E_{AC}(t) \end{pmatrix} = \begin{pmatrix} \alpha_1 \\ \beta_1 \end{pmatrix} \mathrm{e}^{-ir_1 t} \int_0^t dt' F(-t') e^{i(r_1 - \omega_{EE})t'} + \begin{pmatrix} \alpha_2 \\ \beta_2 \end{pmatrix} \mathrm{e}^{-ir_2 t} \int_0^t dt' F(-t') e^{i(r_2 - \omega_{EE})t'} \tag{S33}$$

where $r_1$ and $r_2$ are the eigenvalues of the matrix in eq. (S32) and $\alpha_1, \alpha_2, \beta_1$ and $\beta_2$ are constants that depend on the system parameters. We can now solve for $\phi_A(x,t)$ and $\phi_C(x,t)$ for $t > x > 0$. Note that, when starting in the state described in eq. (S30), the terms proportional to $\theta(-x)\theta(t-x)$ in eqs. (S27) cancel each other. Therefore, for $t > x > 0$ we need to solve the same equations that we had for $x < 0$,

$$\begin{cases} \partial_t \phi_A(x,t) = -\partial_x \phi_A(x,t) - i\left(\omega_A - iV_A^2/2\right)\phi_A(x,t) - i\tilde{J}\phi_C(x,t), \\ \partial_t \phi_C(x,t) = -\partial_x \phi_C(x,t) - i\left(\omega_C - iV_C^2/2\right)\phi_C(x,t) - i\tilde{J}\phi_A(x,t), \end{cases} \tag{S34}$$

but with the boundary conditions given by eq. (S28), where $\phi_{A/C}(0^-,t) = \frac{\pm V_{C/A}}{\sqrt{V_C^2 + V_A^2}} e^{-i\omega_{EE}t} F(-t)$. By applying the Fourier transform to the system in eq. (S34), it can be easily shown that the general solution has the form

$$\phi_A(x>0,t)=\frac{1}{\sqrt{V_C^2+V_A^2}}\left[V_C C_1(x-t)e^{-i\omega_{EE}t}+V_A C_2(x-t)e^{-i\omega_B t}e^{-\Gamma t}\right]$$
$$\phi_C(x>0,t)=\frac{1}{\sqrt{V_C^2+V_A^2}}\left[-V_A C_1(x-t)e^{-i\omega_{EE}t}+V_C C_2(x-t)e^{-i\omega_B t}e^{-\Gamma t}\right] \quad \text{(S35)}$$

where $C_1(x-t)$ and $C_2(x-t)$ are functions to be determined in order to satisfy the boundary conditions in eqs. (S28), and $\omega_B$ and $\Gamma$ are the frequency and the decay rate of the bright single-photon eigenstate of the atom-cavity system.

We now seek for conditions for which, when a single photon impinges on an excited EE, the EE is completely released. That is, only the two-photon probability amplitude $\chi(x_1,x_2,t)$ is nonzero for $t\to+\infty$. The functions $E_{2C}(t)$ and $E_{AC}(t)$ will always decay to zero for $t\to+\infty$, because an EE does not exist in the two-excitation sector of the atom-cavity system. Therefore, we only need to ensure that $\phi_{A/C}(x,t)\to 0$ for $t\to+\infty$. The terms proportional to $C_2(x-t)$ in eqs. (S35) decay to zero for $t\to+\infty$ because $\Gamma\in\mathbb{R}$ and $\Gamma>0$. We therefore conclude that a necessary condition to ensure that $\phi_{A/C}(x,t)\to 0$ is that $C_1(z)=0$ for every $z\equiv x-t<0$ . We note that it is not sufficient to require that $C_1(z)\propto e^{\gamma z}$ with $\gamma>0$, because all the points $x\approx t$ will not experience any decay for $t\to+\infty$.

By applying the boundary conditions in eqs. (S28) to eqs. (S35) we find that

$$C_1(z)=\sqrt{V_C^2+V_A^2}F(z)+\int_0^z dz'\left(\alpha e^{i(r_1-\omega_{EE})(z-z')}+\beta e^{i(r_2-\omega_{EE})(z-z')}\right)F(z') \quad \text{(S36)}$$

where $\alpha$ and $\beta$ are constants that depend on the system parameters. Requiring that $C_1(z)=0$ leads to the Volterra homogeneous equation

$$F(z)=\int_0^z dz' K(z-z')F(z') \quad \text{(S37)}$$

which, for a continuous kernel $K(z-z')$ (as in this case), admits only the trivial solution $F(z)=0$ [6]. We therefore conclude that it is not possible to find a pulse shape $F(x)$ for the initial single-photon pulse such that only a two-photon state is present for $t\to\infty$. However, it can be easily shown that if, for example, $F(x)\propto \exp[-(x-x_0)^2/(2\sigma^2)+ikx]$, equation (S37) can be satisfied with arbitrarily high accuracy as $\sigma\to\infty$. That is, we can obtain final states arbitrarily close to a two-photon state by working with larger and larger impinging pulses.

## References


[1] S. Fan, Ş. E. Kocabaş, and J. T. Shen, "Input-output formalism for few-photon transport in one-dimensional nanophotonic waveguides coupled to a qubit," *Phys. Rev. A - At. Mol. Opt. Phys.*, vol. 82, no. 6, 2010.

[2] H. Friedrich and D. Wintgen, "Interfering resonances and bound states in the continuum," *Phys.*

*Rev. A*, vol. 32, no. 6, pp. 3231–3242, 1985.

[3] J. R. Johansson, P. D. Nation, and F. Nori, “QuTiP 2: A Python framework for the dynamics of open quantum systems,” *Comput. Phys. Commun.*, vol. 184, no. 4, pp. 1234–1240, 2013.

[4] Y.-L. L. Fang, F. Ciccarello, and H. U. Baranger, “Non-Markovian dynamics of a qubit due to single-photon scattering in a waveguide,” *New J. Phys.*, vol. 20, no. 4, p. 43035, Apr. 2018.

[5] Y.-L. L. Fang, “FDTD: solving 1+1D delay PDE,” *arXiv:1707.05943 [physics, physics:quant-ph]*, 2017.

[6] A. D. Polyanin, And, and A. V. Manzhirov, *Handbook of Integral Equations*. 1998.
